# Supplementary material for: TallyQA: Answering Complex Counting Questions
Source: arXiv:1810.12440 source file (2018-10-31)
Supplement: Supplementary file 1 [file supp.tex]

\section{Supplementary Material}
\begin{figure*}[t]
\centering
\footnotesize
    \captionsetup[subfigure]{justification=centering}    
        \begin{subfigure}[t]{0.3\textwidth}
		\includegraphics[width=\textwidth, ]{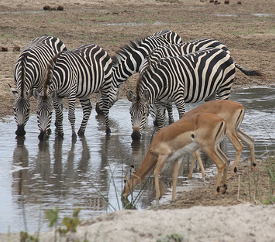}
        \caption{
	    How many zebras are there? 
        \textcolor{green}{GT}: 5}
    \end{subfigure}
    \hfill
    \begin{subfigure}[t]{0.3\textwidth}
	 	\includegraphics[width=\textwidth, ]{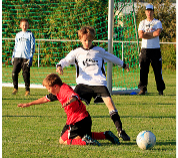}
        \caption{
	    How many people are pictured?
        \textcolor{green}{GT}: 4 }
	\end{subfigure}
    \hfill
    \begin{subfigure}[t]{0.3\textwidth}
	 	\includegraphics[width=\textwidth, ]{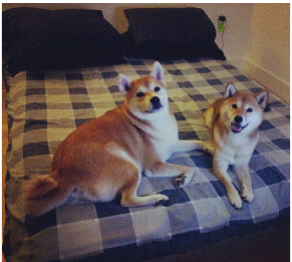}
\caption{How many dogs are there?
        \textcolor{green}{GT}: 2 }
\end{subfigure}
        \begin{subfigure}[t]{0.3\textwidth}
		\includegraphics[width=\textwidth, ]{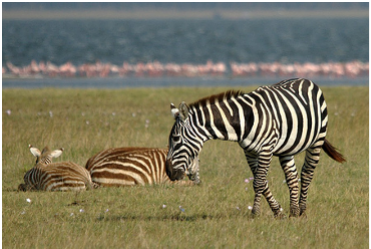}
        \caption{
	    How many zebras are standing in this image? 
\textcolor{green}{GT}: 1 }
    \end{subfigure}
    \hfill
    \begin{subfigure}[t]{0.3\textwidth}
	 	\includegraphics[width=\textwidth, ]{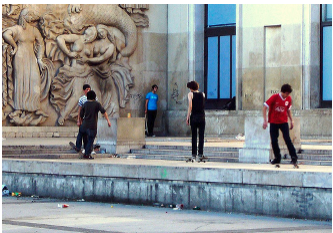}
        \caption{
	    How many people are not wearing red shirts?
        \textcolor{green}{GT}: 4}
	\end{subfigure}
    \hfill
    \begin{subfigure}[t]{0.3\textwidth}
	 	\includegraphics[width=\textwidth, ]{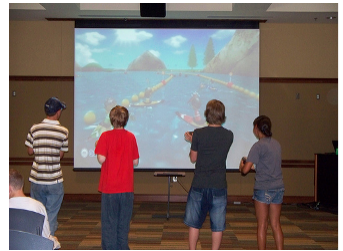}
\caption{How many people wear hat?
       \textcolor{green}{GT}: 1 }
\end{subfigure}
\caption{Simple (top row) and Complex (bottom row) questions with their Ground Truth (GT) answers in TallyQA.}
\label{fig:simpcomp}
    \end{figure*}

\newpage
\begin{figure*}[b]
  \centering
    \includegraphics[scale=0.52,keepaspectratio]{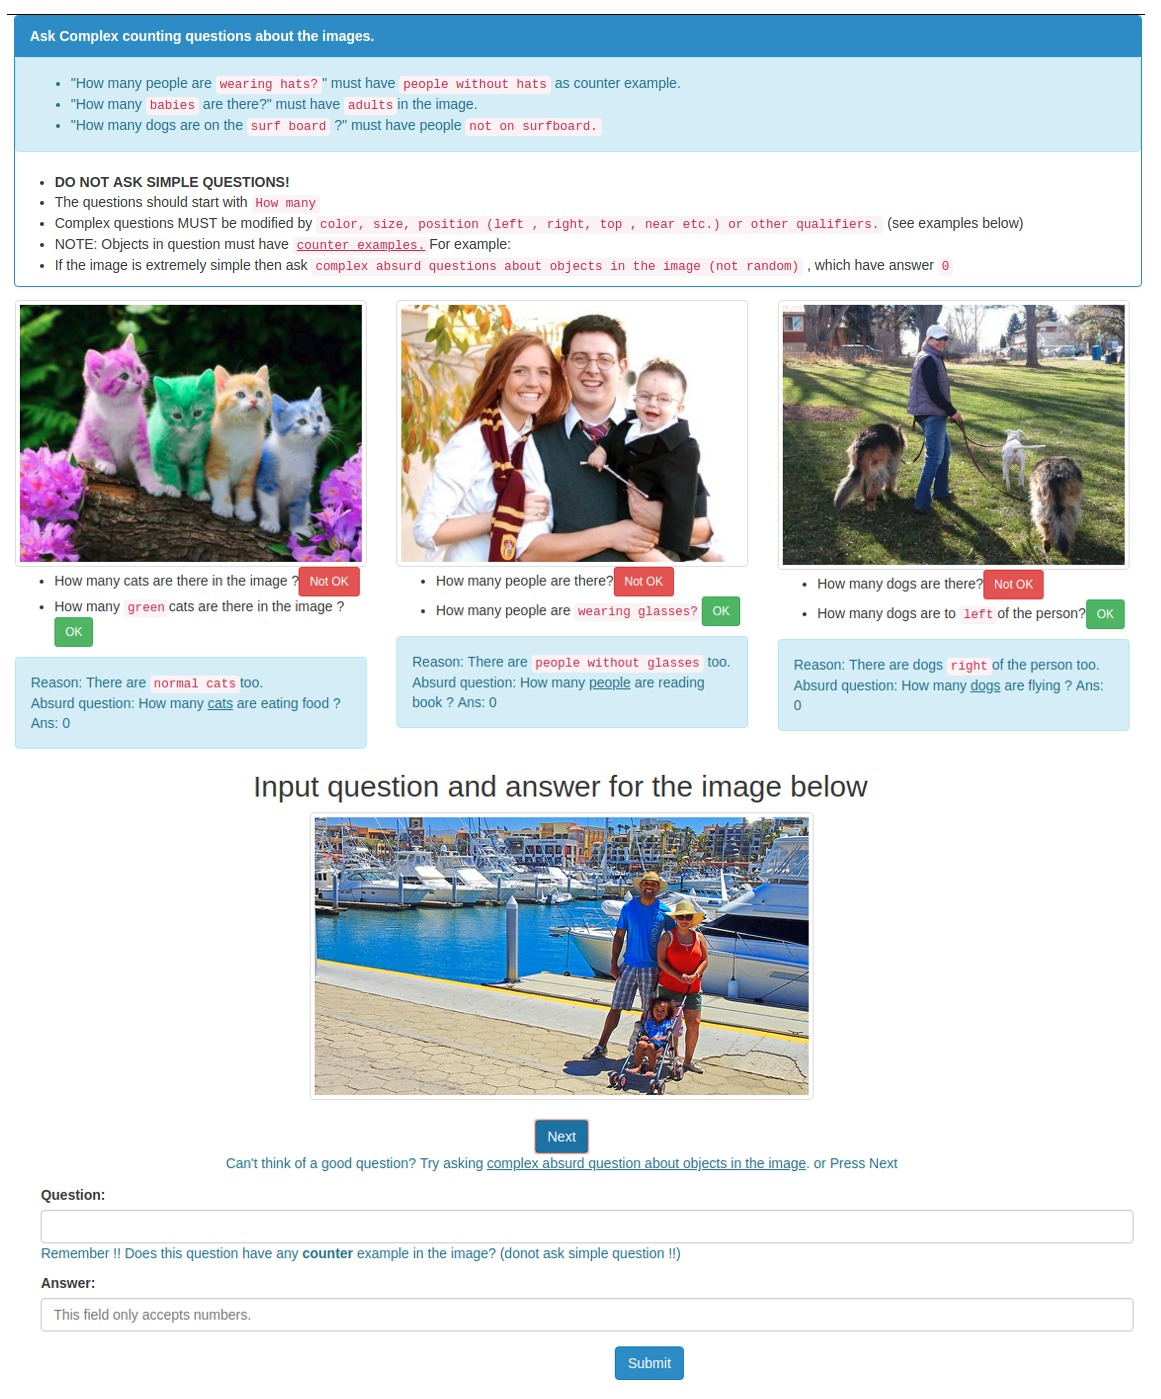}     
\caption{ AMT web data collection interface for TallyQA dataset. }
% Snap shot of our interface like in visual dialog paper https://arxiv.org/pdf/1611.08669.pdf  }  
\label{fig:interface}
\end{figure*}
